# Supplementary material for: PAAM: A Framework for Coordinated and Priority-Driven Accelerator Management in ROS 2
Source: arXiv:2404.06452 source file (2024-04-09)
Supplement: Supplementary file 1 [file appendix.tex]

\newpage
\label{sec:appendix}
\appendix
\input{draft/5-Analysis-Long}
